# Supplementary material for: CADyQ: Content-Aware Dynamic Quantization for Image Super-Resolution
Source: arXiv:2207.10345 source file (2022-10-30)
Supplement: Supplementary file 1 [file sup-measure.tex]

\begin{table*}[h!]
\centering
\caption{ \textbf{Ablation study on quantization sensitivity measures.}
\textcolor{blue}{remove overlapping contents with the main text}
Evaluation is conducted with CARN as a backbone, on Urban100.
}
\scalebox{0.99}{
    \begin{tabular}{@{}c|ccccc}
        \toprule
        & Patch & Layer & $\text{FQR}_\downarrow$ & $\text{PSNR}_\uparrow$ & $\text{SSIM}_\uparrow$\\
        \midrule
        \textbf{(S4a)} & std & layer std & 5.95 & 25.62 & 0.769 \\
        \textbf{(S4b)} & gradient & layer std & 6.53 & 25.80 & 0.775 \\
        \rowcolor{orange!25}
        \textbf{CADyQ} & gradient & channel std & 5.32 & 25.94&0.780\\
        \bottomrule
    \end{tabular}
}
\label{tab:sup-measure}
\end{table*}
